# Supplementary material for: Anisotropy and controllable band structure in supra-wavelength polaritonic metasurfaces
Source: arXiv:1903.03328 ancillary file (2019-03-08)
Supplement: Supplementary file 1 [file SMChevrierArxiv.pdf]

# Supplementary Material for:

# **Anisotropy and controllable band structure in supra-wavelength polaritonic metasurfaces**

K. Chevrier[1], J.M. Benoit[1], C. Symonds[1], S. Saikin[2], J. Yuen Zhou[3], J. Bellessa[1]*

*1 Univ. Lyon, Université Claude Bernard Lyon 1, CNRS, Institut Lumière Matière, F-69622, LYON, France.*

*2 Department of Chemistry and Chemical Biology, Harvard University, Cambridge, MA 02138, USA.*

*3 Department of Chemistry and Biochemistry, University of California San Diego, La Jolla, CA, USA.*

## **Absorption of the TDBC and UV-irradiated TDBC films**

The Figure 1 presents the absorption spectra recorded on a TDBC thin film, and on a UV-irradiated TDBC thin film. On the bare TDBC film; the absorbance is measured at 2.1 eV ($\lambda$ = 590 nm) as expected for TDBC. After UV-irradiation, the absorption of the TDBC vanishes showing the bleaching of the film.

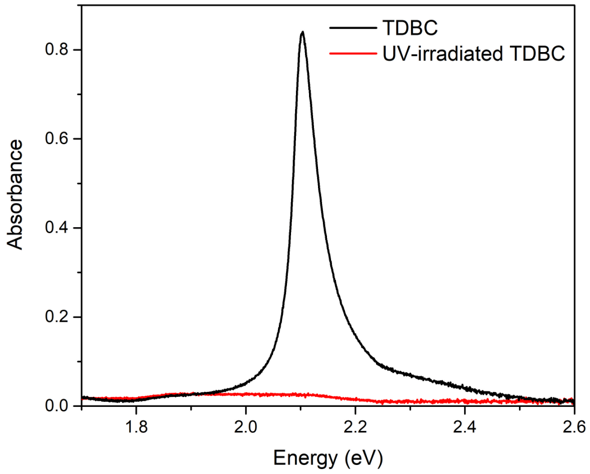


**Figure 1:** Absorbance spectra of a TDBC thin film (black line) and an UV-irradiated TDBC thin film (red line)

## Propagation length measurement

The polariton coherence length is of the same order of magnitude as the polariton propagation length[1]. This length can be deduced from the wavevector broadening Δk of the polaritonic line (measured at constant energy) in the dispersion image. For a Lorentzian shape, with a full width at half maximum Δk, the Fourier transform is an exponential decay with a characteristic length equal to 2/Δk. As the dispersion image (recorded in the Fourier plane of the collection lens) is the Fourier transform of the direct image, we can deduce the propagating length of the polaritons[2] $\ell$=2/Δk. For the uniform dye layer on silver, the full width at half maximum at constant wavelength is Δk=0.289µm$^{-1}$ at λ=614.5nm, giving a polariton extension of 7µm.

## Quantum mechanical description of polariton metasurfaces

We elaborate on the quantum theoretical formalism that is outlined in the main text. The starting point is a model of the metasurface as a two-dimensional lattice (we take $\hbar = 1$) whose real space description is given by

$$H' = \sum_{k} \omega_k a_k^\dagger a_k + \sum_{n,v} \omega_v \sigma_{n,v}^\dagger \sigma_{n,v} + \sum_{k,n,v} \left[ g_{k,v} e^{ik_x(x_n+va)+ik_y y_n} \sigma_{n,v}^\dagger a_k + h.c. \right] \ldots (S1)$$

This expression comprises $N_{cells} \times N$ unit cells of dimension $L \times a$ labeled by the Cartesian pair $n = (n_x, n_y)$. Here, $L = N_{uc} a$ is the patterning period, $N_{uc}$ is the number of lattice points in the unit cell, and $a \ll L$ is the smallest spatial resolution of the simulation which, owing to our emphasis in microscale phenomena, is conveniently taken to be much larger than the nanoscale intermolecular distance. Operators $\sigma_{n,v}^\dagger (\sigma_{n,v})$ describe the creation (annihilation) of an exciton in an isotropically polarizable molecular unit with coordinates $(n_x L + va, n_y a)$. This exciton shall be regarded as a coarse-

grained representation of the collective bright exciton delocalized across an $a \times a$ in-plane area of the film[i]. It is characterized by an energy $\omega_v = \omega_e p_v + \omega_h(1 - p_v)$, where $\omega_e$ is the molecular transition frequency of the active dye aggregate[ii] while $\omega_h \to \infty$ is the corresponding one for the photobleached dye. $p_v$ is the patterning function such that $p_v = 1$ for $v = 0, \cdots, fN_{uc} - 1$ and $p_v = 0$ otherwise, where $f$ is the filling factor. $a_k^\dagger(a_k)$ describes the creation (annihilation) of a bosonic excitation ($[a_k, a_k^\dagger] = \delta_{k,k'}$) at the surface plasmon labeled by wavevector $k = (k_x, k_y) = \frac{2\pi}{Na}(s_x, s_y)$ with integers $s_i \in \left[-\frac{N}{2}, \frac{N}{2}\right)$. $g_{k,v} = g_k p_v$ is a coarse-grained amplitude of light-matter coupling, which is determined by enforcing it to yield the same polariton dispersion as the real three-dimensional metasurface.

Given the considerations above, the shortcut notation is defined as follows,

$$\sum_n = \sum_{n_x=0}^{N_{cells}-1} \sum_{n_y=0}^{N-1},$$

$$\sum_v = \sum_{v=0}^{N_{uc}-1},$$

$$\sum_k = \sum_{k_x=\frac{2\pi s_x}{Na}} \sum_{k_y=\frac{2\pi s_y}{Na}} = \sum_{s_x=-\frac{N}{2}}^{\frac{N}{2}-1} \sum_{s_y=-\frac{N}{2}}^{\frac{N}{2}-1}.$$

To be specific, we hereafter focus on the case of ½ filling factor; generalization to other factors is straightforward. Eq. (S1) can be block-diagonalized in Fourier space, $H' = H + H_h$ where $H_h = \omega_h \sum_n \sum_{v=\frac{N_{uc}}{2}}^{N_{uc}-1} \sigma_{n,v}^\dagger \sigma_{n,v}$ refers to high-lying off-resonant molecular excitations in the photobleached

[i] Given that $H'$ is a two-dimensional coarse-graining of a three-dimensional structure, it does not properly describe dark or reservoir states which correspond to exciton superpositions that feature one or more nodes along the $z$ direction and which, owing to symmetry, do not couple to plasmons[10,11]. These states do not affect the linear optical properties of the metasurfaces, but will be important for the description of nonlinear properties.

[ii] $\omega_e$ is the transition frequency which already includes a renormalization to the bare molecular energy arising from dipolar couplings between chromophores in the aggregate.

stripes, which we can ignore for purposes of understanding the low-energy excitations, and $H=\sum_K H_K$, with $H_K$ expressed in Eq. (1) of the main text, which we reproduce here for completeness,

$$H_K=\sum_{\kappa}\omega_{K+\kappa}a^{\dagger}_{K+\kappa}a_{K+\kappa}+\omega_e\sum_{\kappa'}{}' \sigma^{\dagger}_{K+\kappa'}\sigma_{K+\kappa'}+\sum_{\kappa}\sum_{\kappa'}{}' [J_{K+\kappa}F_{\kappa-\kappa'}\sigma^{\dagger}_{K+\kappa'}a_{K+\kappa}+h.c.] \dots (S2)$$

From Eq. $(S2)$, it is evident that the supra-wavelength patterning renders the domain of $K$ a reduced Brillouin zone (compared to the domain of $k$), $K=(K_x,K_y)=(K_x,k_y)=\frac{2\pi}{Na}(m_x,s_y)$ with integer $m_x\in[0,N_{cells})$. The wavevectors $k$ of the original Brillouin zone can be uniquely related to this reduced Brillouin zone by virtue of the unique decomposition $k=K+\kappa$, where $\kappa=(\kappa_x,0)$ is a Bragg vector [$\kappa_x=\frac{2\pi\bar{m}_x}{N_{uc}a}$ and integer $\bar{m}_x\in\left[-\frac{N_{uc}}{2},\frac{N_{uc}}{2}\right)$]. A check of this decomposition consists on noticing that there are $N_{cells}\times N$ and $N_{uc}$ possible values for $K$ and $\kappa$, respectively, giving the same count as the original number of $k$ points (and therefore, of plasmon modes in the simulation), $N_{cells}NN_{uc}=N^2$.

On the other hand, the active dye exciton operators in Fourier space read as,

$$\sigma^{\dagger}_{K+\kappa'}=\frac{1}{\sqrt{\frac{N_{uc}}{2}}}\sum_{v=0}^{\frac{N_{uc}}{2}-1}e^{i\kappa_x' va}\,\frac{1}{\sqrt{N_{cells}N}}\sum_{n}e^{iK_x(n_xL+va)+ik_yn_ya}\sigma^{\dagger}_{n,v}\,, \dots (S3)$$

with $\kappa'=(\kappa_x',0)=\frac{2\pi\bar{m}_x'}{N_{uc}a}$ and *even* integer $\bar{m}_x'\in\left[-\frac{N_{uc}}{2},\frac{N_{uc}}{2}\right)$. Given the parity condition for $\bar{m}_x$, there are only $\frac{N_{uc}}{2}$ possible values for $\kappa'$, giving rise to the original number of active dye exciton operators $N_{cells}N\frac{N_{uc}}{2}=\frac{N^2}{2}$. To summarize, the $K$ decomposition of $H$ gives rise to $N_{cells}\times N$ Hamiltonians $H_K$, each of which can be represented as an $\left(\frac{N_{uc}}{2}+N_{uc}\right)\times\left(\frac{N_{uc}}{2}+N_{uc}\right)$ matrix. The size of these matrices can also be rationalized from the composition of the unit cells ( $\frac{N_{uc}}{2}$ active-dye units and $N_{uc}$ lattice points where the plasmon mode electric fields can take finite values). Only plasmon and exciton

operators whose wavevectors differ by a Bragg vector can mix according to the Fourier transform of the patterning function, $F_{\Delta\kappa} = \frac{\sqrt{2}}{N_{uc}} \sum_{v=0}^{N_{uc}-1} p_v e^{i\Delta\kappa v a}$, which can be explicitly evaluated to yield,

$$F_{\kappa-\kappa'} = \frac{1}{\sqrt{2}} \delta_{\kappa,\kappa'} + \delta_{(\bar{m}_x - \bar{m}'_x),1}^{(mod\ 2)} \times \frac{\sqrt{2}}{N_{uc}} \times \frac{i}{e^{\frac{i\pi(\bar{m}_x - \bar{m}'_x)}{N_{uc}}} \sin \frac{\pi(\bar{m}_x - \bar{m}'_x)}{N_{uc}}} . \dots (S4)$$

Here, $\delta_{x,y}^{(mod\ 2)} = 1$ if $x \equiv y\ (mod\ 2)$ and $0$ otherwise. Eq. $(S2)$ conveniently expresses the collective light-matter interaction in terms of $F_{\kappa-\kappa'}$ and the isotropically averaged collective coupling of the film in the absence of patterning. This coupling is given by[3–6] $J_k = \sqrt{\rho \int_{z_0}^{z_f} \left[ \frac{2}{3} \left| J_k^{(x)}(z') \right|^2 + \frac{1}{3} \left| J_k^{(z)}(z') \right|^2 \right] dz'}$ and formally equivalent to $J_k = \sqrt{N^2} g_{k,0}$ (there are $N^2$ polarizable units in the simulation in the absence of patterning). Here, $z_0$ and $z_f$ are the $z$ coordinates corresponding to the bottom and top of the molecular layer on top of the metal-dielectric interface ($z = 0$), $\rho$ is the density of chromophores in the molecular layer, $J_k^{(i)}(z) = \sqrt{\frac{\omega_k}{2\epsilon_0 L_k}} |\mu|\, \hat{\imath} \cdot E_k e^{-\alpha_{dk} z}$ is a $z$-dependent evanescent plasmon-exciton coupling[6], $\mu$ is the single-molecule transition dipole moment, $\omega_k = c|k| \sqrt{\frac{\epsilon_d + \epsilon_m}{\epsilon_d \epsilon_m}}$ is the plasmon frequency ($\epsilon_d$ is the dielectric permittivity of the dye, $\epsilon_m = \epsilon_\infty - \frac{\omega_p^2}{\omega^2}$ is the Drude permittivity of the metal), $E_k = \left(1, 0, \frac{ik}{\alpha_{dk}}\right)$ is the electric field profile, and $\alpha_{sk} = -i\sqrt{\frac{\epsilon_s \omega_k^2}{c^2} - |k|^2}$ is the evanescent decay constant of the plasmon in the $s = d, m$ (dielectric, metal) layer[7]. $L_k$ is the plasmonic quantization length[3,5,6]

$$L_k = -\frac{\epsilon_m}{\alpha_{dk}} + \frac{1}{2\alpha_{mk}} \left\{ \left[ \frac{d\big(\omega \epsilon_m(\omega)\big)}{d\omega} \right]_{\omega_k} \frac{(\epsilon_m - \epsilon_d)}{\epsilon_m} - \epsilon_m - \epsilon_d \right\} . \dots (S3)$$

## Numerical simulations.

Numerical diagonalization of $H_K$ for all $K$ points affords a simulation of the plasmon-weighted polariton metasurface dispersion $I_{plasmon}$. In particular, we define discrete grids for wavevector $k \in \left[-\frac{\pi}{a}, \frac{\pi}{a}\right) \times \left[-\frac{\pi}{a}, \frac{\pi}{a}\right)$ (extended Brillouin zone) and energy $\omega \in [0{,}3\, eV]$. For every pair $(k, \omega)$, we compute $I_{plasmon}(k, \omega) = \sum_{K,j} \left|\alpha_k^{K;j}\right|^2 \bar{\delta}_{\omega,\omega^{K;j}}$, where the jth eigenstate and eigenvalue of $\mathrm{H_K}$ are given by $\zeta^{K;j\dagger} = \sum_k (\alpha_k^{K;j}\, a_k^{+} + \beta_k^{K;j} \sigma_k^{+})$ and $\omega^{K;j}$, respectively, and $\bar{\delta}_{\omega,\omega'}$ is a binning function to collect signal in the corresponding energy bin ($\bar{\delta}_{\omega,\omega'} = 1$ if $\omega' \in [\omega, \omega + \Delta)$ and $\bar{\delta}_{\omega,\omega'} = 0$ otherwise, where $\Delta$ is the resolution of the energy grid). Calculation of the eigenstates of $H_K$ in the $\{a_k^{\dagger}, \sigma_k^{\dagger}\}$ plane-wave basis allows for the reconstruction of the real-space plasmon and exciton densities by the corresponding weighted coherent superposition of plane-wave amplitudes (see Fig. 3).

Table SM-1 summarizes the values of parameters used in the simulations.

| TABLE SI-1. PARAMETERS USED IN SIMULATIONS | | | |
|---|---|---|---|
| | PARAMETER | VALUE | NOTES |
| Drude model for Ag | $\epsilon_\infty$ | $3.7$ | [8] |
| | $\omega_P$ | $8.6\ eV$ | [8] |
| | $c$ | $3 \times 10^8\ m/s$ | |
| Molecular layer | $\epsilon_d$ | $1.07$ | Value chosen to optimize fit with the experimental dispersion of the bare plasmon given $\epsilon_\infty$, $\omega_P$, and $c$ above. |
| | $\omega_e$ | $2.06\ eV$ | Experimental fit. |
| | $z_0$ | $1\ nm$ | Experimental value. |
| | $z_f$ | $18\ nm$ | Experimental value. |
| | $\mu$ | $10\ Debye$ | [9] |
| | $\rho$ | $4 \times 10^8 \frac{molecules}{\mu m^3}$ | Value chosen to optimize fit with the experimental Rabi splitting at resonance given the parameters above. |
| Real space Coarse-graining | $N$ | $\sim 1500 - 15000$ | The coarse-grained grid was defined so that $\max(\lvert k_x \rvert) = \frac{\pi}{a} > 15\ \mu m^{-1}$, which is the largest experimentally measured wavevector in the reported experiments. This means that the real-space lattice spacing is $a = \frac{\pi}{\max(\lvert k_x \rvert)} < 0.2\ \mu m$. Next, $N_{uc} = \frac{L}{a}$ is taken to be even (to properly simulate the patterning at half-filling). Finally, the $k_x$ grid resolution was fixed at $\Delta k = \frac{2\pi}{Na} \approx 0.02\ \mu m^{-1}$. These constraints yield the number of unit cells $N \times N_{cells}$ where $N_{cells} = \frac{N}{N_{uc}}$. |

(1) S. Aberra Guebrou, C. Symonds, E. Homeyer, J.C. Plenet, Y.N. Gartstein, V.M. Agranovich and J. Bellessa, Phys. Rev. Lett. **108**, 066401 (2012).

(2) K. Chevrier, J.M. Benoit, C. Symonds, J. Paparone, J. Laverdant and J.Bellessa, ACS Photonics **5,** 80-84 (2018).

(3) A. Archambault, F. Marquier, J.J. Greffet and C. Arnold, Phys. Rev. B **82**, 35411 (2010).

(4) A. Gonzalez-Tudela, P.A. Huidobro, L. Martin-Moreno, C. Tejedor and F.J. Garcia-Vidal, Phys. Rev. Lett. **110**, 114018 (2013).

(5) J. Yuen-Zhou, S.K. Saikin, T. Zhu, M.C. Onbasli, C.A. Ross, V. Bulovic and M.A. Baldo, Nat. Comm. **7**, 11783 (2016).

(6) J. Yuen-Zhou, S.K. Saikin and V. Menon, *Plexciton Photoluminescence: Van Hove Anomalies and Superradiance*, *arXiV:1711.11213* (2017).

(7) S.A. Maier, *Plasmonics: Fundamentals and Applications* (Springer, 2007).

(8) P.R. West, S. Ishii, G.V. Naik, N.K. Emani, V.M. Shalaev and A. Boltasseva, Laser Photon. Rev. **4**, 795–808 (2010).

(9) S.K. Saikin, A. Eisfeld, S. Valleau and A. Aspuru-Guzik, Nanophotonics **2**, 21–38 (2013).

(10) V.M. Agranovich, M. Litinskaia and D.G. Lidzey, Phys. Rev. B **67**, 85311 (2003).

(11) R.F. Ribeiro, L.A. Martínez-Martínez, M. Du, J. Campos-Gonzalez-Angulo, J. Yuen-Zhou, *Polariton Chemistry: Controlling Molecular Dynamics with Optical Cavities*, Chem. Sci. **9**, 6325-6339 (2018).
